# Supplementary material for: Comparing Perturbative and Commutator-Rank-Based Truncation Schemes in Unitary Coupled-Cluster Theory
Source: arXiv:2503.00617 ancillary file (2025-05-02)
Supplement: Supplementary file 1 [file unitary_cc_si.pdf]

# Supporting Information for: Comparing Perturbative and Commutator-Rank-Based Truncation Schemes in Unitary Coupled-Cluster Theory

Justin T. Phillips, Lauren N. Koulias, Stephen H. Yuwono, and A. Eugene DePrince III[a)]
*Department of Chemistry and Biochemistry, Florida State University, Tallahassee, FL 32306-4390*

TABLE I. Equilibrium bond lengths of the small molecules examined in this work.

| Molecule | $R_e$ (Å) |
|---|---|
| HF | 0.91680 |
| $H_2O$ | 0.958[a] |
| $N_2$ | 1.09768 |
| CO | 1.128323 |
| $F_2$ | 1.41193 |

[a] H–O–H angle = 104.5°.

[a)]Electronic mail: adeprince@fsu.edu

TABLE II. Errors in the PEC of the $C_{2v}$ Be + $H_2$ insertion reaction obtained using CCSD and the UCC methods reported in Fig. 1 relative to the full CI data (in mEh). The full CI energy is reported in Eh.

| $x$ ($a_0$) | CCSD | UCCSD(4) | UCCSD(5) | BCH (rank 3) | BCH (rank 4) | Bernoulli (rank 3) | Bernoulli (rank 4) | FCI |
|---|---|---|---|---|---|---|---|---|
| 0.00 | 0.625 | 0.508 | 0.611 | 0.802 | 0.793 | 0.420 | 0.624 | −15.836415 |
| 0.25 | 0.596 | 0.475 | 0.584 | 0.770 | 0.761 | 0.399 | 0.595 | −15.833855 |
| 0.50 | 0.585 | 0.465 | 0.575 | 0.759 | 0.750 | 0.392 | 0.585 | −15.826337 |
| 0.75 | 0.590 | 0.478 | 0.581 | 0.767 | 0.758 | 0.397 | 0.593 | −15.815623 |
| 1.00 | 0.610 | 0.516 | 0.602 | 0.794 | 0.785 | 0.415 | 0.617 | −15.803362 |
| 1.25 | 0.648 | 0.581 | 0.640 | 0.843 | 0.833 | 0.447 | 0.661 | −15.790233 |
| 1.50 | 0.712 | 0.681 | 0.704 | 0.924 | 0.913 | 0.498 | 0.733 | −15.775702 |
| 1.75 | 0.814 | 0.828 | 0.806 | 1.055 | 1.042 | 0.572 | 0.847 | −15.758539 |
| 2.00 | 0.974 | 1.036 | 0.966 | 0.674 | 1.026 | 1.258 | 1.243 | −15.737632 |
| 2.05 | 1.015 | 1.085 | 1.007 | 0.697 | 1.073 | 1.310 | 1.295 | −15.732953 |
| 2.10 | 1.062 | 1.139 | 1.053 | 0.720 | 1.124 | 1.369 | 1.352 | −15.728110 |
| 2.15 | 1.112 | 1.195 | 1.103 | 0.743 | 1.180 | 1.432 | 1.414 | −15.723106 |
| 2.20 | 1.167 | 1.253 | 1.158 | 0.763 | 1.241 | 1.500 | 1.483 | −15.717948 |
| 2.25 | 1.230 | 1.315 | 1.220 | 0.781 | 1.310 | 1.577 | 1.559 | −15.712646 |
| 2.30 | 1.299 | 1.379 | 1.288 | 0.793 | 1.387 | 1.662 | 1.643 | −15.707212 |
| 2.35 | 1.380 | 1.446 | 1.368 | 0.796 | 1.476 | 1.758 | 1.740 | −15.701663 |
| 2.40 | 1.474 | 1.516 | 1.461 | 0.782 | 1.579 | 1.869 | 1.852 | −15.696020 |
| 2.45 | 1.588 | 1.587 | 1.574 | 0.737 | 1.705 | 1.999 | 1.986 | −15.690312 |
| 2.50 | 1.735 | 1.659 | 1.720 | 0.622 | 1.865 | 2.161 | 2.153 | −15.684580 |
| 2.55 | 1.932 | 1.738 | 1.917 | 0.231 | 2.080 | 2.369 | 2.374 | −15.678881 |
| 2.60 | 2.212 | — | 2.201 | 2.016 | 2.388 | 2.654 | 2.681 | −15.673301 |
| 2.65 | 2.642 | — | 2.641 | −7.649 | 2.861 | 3.072 | 3.141 | −15.667981 |
| 2.70 | 3.344 | — | 3.372 | 3.782 | 3.642 | 3.723 | 3.877 | −15.663156 |
| 2.75 | 4.542 | — | 4.644 | 26.857 | 4.994 | 4.762 | 5.102 | −15.659226 |
| 2.80 | 6.568 | 40.257 | 6.859 | 29.259 | 7.346 | 6.279 | 7.101 | −15.656806 |
| 2.85 | 9.096 | 43.257 | 10.120 | 24.191 | 10.971 | 8.365 | 9.479 | −15.656540 |
| 2.90 | 6.385 | 49.155 | 6.794 | 21.784 | 7.468 | 6.988 | 7.297 | −15.658574 |
| 2.95 | 4.683 | 57.309 | 4.812 | 17.738 | 5.360 | 5.593 | 5.644 | −15.662387 |
| 3.00 | 3.661 | 66.919 | 3.658 | 15.951 | 4.119 | 4.622 | 4.587 | −15.667300 |
| 3.05 | 3.031 | 77.383 | 2.964 | 17.897 | 3.363 | 3.978 | 3.910 | −15.672828 |
| 3.10 | 2.618 | 88.296 | 2.523 | −10.116 | 2.875 | 3.537 | 3.456 | −15.678682 |
| 3.15 | 2.331 | 99.384 | 2.225 | 18.620 | 2.541 | 3.218 | 3.134 | −15.684698 |
| 3.20 | 2.119 | 110.441 | 2.010 | −1.920 | 2.297 | 2.975 | 2.892 | −15.690775 |
| 3.25 | 1.954 | 121.291 | 1.848 | −4.467 | 2.112 | 2.782 | 2.703 | −15.696851 |
| 3.30 | 1.818 | 131.660 | 1.718 | −3.540 | 1.962 | 2.622 | 2.547 | −15.702878 |
| 3.35 | 1.702 | −0.594 | 1.609 | −1.936 | 1.836 | 2.484 | 2.414 | −15.708820 |
| 3.40 | 1.601 | −0.474 | 1.516 | −1.706 | 1.728 | 2.363 | 2.298 | −15.714646 |
| 3.45 | 1.509 | −0.401 | 1.433 | −1.471 | 1.631 | 2.253 | 2.194 | −15.720324 |
| 3.50 | 1.425 | −0.365 | 1.357 | −1.327 | 1.543 | 2.154 | 2.099 | −15.725823 |
| 3.55 | 1.347 | −0.352 | 1.286 | −1.233 | 1.461 | 2.061 | 2.011 | −15.731109 |
| 3.60 | 1.273 | −0.356 | 1.220 | −1.170 | 1.385 | 1.974 | 1.929 | −15.736145 |
| 3.65 | 1.203 | −0.370 | 1.157 | −1.128 | 1.313 | 1.893 | 1.851 | −15.740890 |
| 3.70 | 1.136 | −0.392 | 1.097 | −1.101 | 1.245 | 1.816 | 1.778 | −15.745297 |
| 3.75 | 1.071 | −0.422 | 1.039 | −1.086 | 1.178 | 1.742 | 1.707 | −15.749311 |
| 3.80 | 1.010 | −0.454 | 0.984 | −1.079 | 1.116 | 1.672 | 1.641 | −15.752874 |
| 3.85 | 0.951 | −0.489 | 0.930 | −1.080 | 1.056 | 1.606 | 1.578 | −15.755914 |
| 3.90 | 0.894 | −0.527 | 0.879 | −1.086 | 0.998 | 1.542 | 1.516 | −15.758351 |
| 3.95 | 0.840 | −0.566 | 0.829 | −1.095 | 0.942 | 1.481 | 1.458 | −15.760093 |
| 4.00 | 0.788 | −0.605 | 0.781 | −1.108 | 0.889 | 1.423 | 1.403 | −15.761033 |
